# Supplementary material for: Massively parallel quantum chemistry: PFAS on over 1 million cloud vCPUs
Source: arXiv:2307.10675 source file (2023-07-20)
Supplement: Supplementary file 1 [file SI.pdf]

# Supplemental Information for
# Massively parallel quantum chemistry: PFAS on over 1 million cloud vCPUs

Alan E. Rask[1], Lee Huntington[1], SungYeon Kim[1], David Walker[1], Andrew Wildman[1], Rodrigo Wang[1], Nicole Hazel[1], Alan Judi[1], James T. Pegg[1], Punit K. Jha[1], Zara Mayimfor[1], Carl Dukatz[2], Hassan Naseri[2], Ilan Gleiser[3], Maxime R. Hugues[3], Paul M. Zimmerman[1,4], Arman Zaribafiyan[1], Rudi Plesch[1*] and Takeshi Yamazaki[1*]

[1]Good Chemistry Company,
200-1285 West Pender Street, Vancouver, V6E 4B1, BC, Canada.
[2]Accenture,
1 Grand Canal Quay, Grand Canal Dock, Dublin, D02 P820, Ireland.
[3]Amazon Web Services,
410 Terry Ave N, Seattle, 98109, Washington, United States.
[4]Department of Chemistry, University of Michigan,
Ann Arbor, 48109, Michigan, United States.

*Corresponding author(s). E-mail(s): rudi@goodchemistry.com; takeshi@goodchemistry.com

Table of Contents

I. 3- and 4-Body Truncation Procedure (CnB)
II. Total Number of *n*-Body Terms Computed
III. Molecular Geometries
IV. References

# I. 3- and 4-Body Truncation Procedure (CnB)

The connected $n$-body procedure (CnB) predicts the magnitude of an $n$-body term from ($n$–1)-body terms according to a cutoff, $\mathscr{C}$.[1,2] Connections between $n$- and ($n$–1)-body terms are made according to orbital indices and if two or more ($n$–1)-body terms are above the chosen cutoff, the $n$-body term is computed. An example scenario for $n = 2–4$ is shown in Figure 1, and a detailed description of this procedure is given in the Supporting Information of Ref. 2 (Section I).

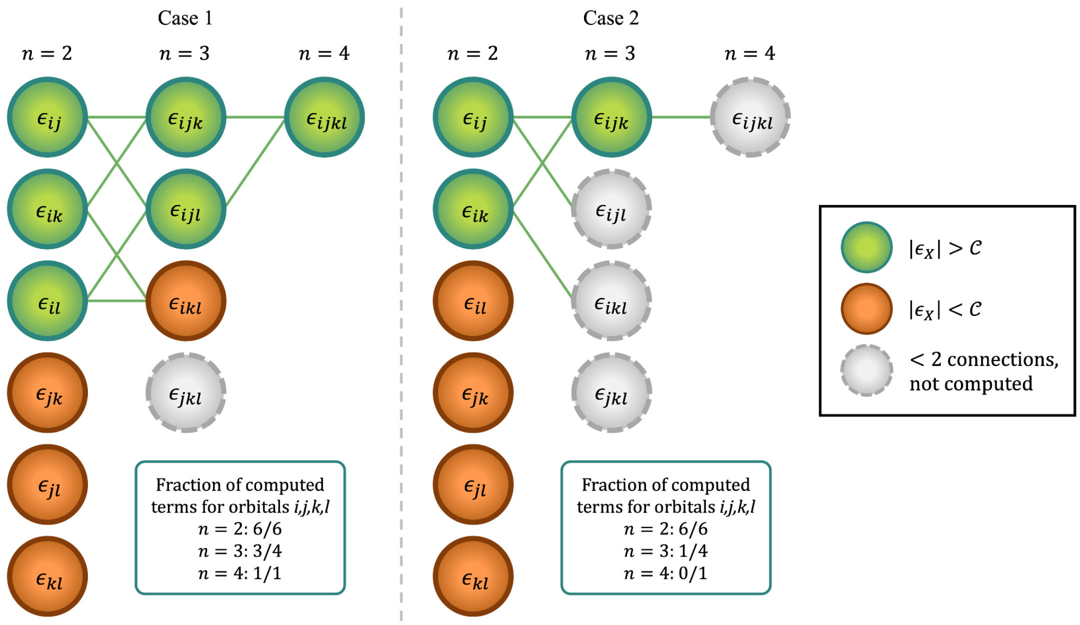


Figure 1) Combinations of orbitals the $i,j,k,l$ produce a set of $n$-body terms that each contribute a different amount of correlation energy ($\epsilon_X$). Moving from lower-to-higher $n$, the magnitude of each ($n$–1)-body term is checked against the cutoff, $\mathscr{C}$, to determine if the $n$-body term should be computed. In example case 1, three 2-body terms are above $\mathscr{C}$ ($\epsilon_{ij}$, $\epsilon_{ik}$, $\epsilon_{il}$), which produce three 3-body terms ($\epsilon_{ijk}$, $\epsilon_{ijl}$, $\epsilon_{ikl}$) that each contain the combination of orbitals of at least two of these 2-body terms (indicated by green connecting lines). The remaining 3-body term ($\epsilon_{jkl}$) is not computed because $\epsilon_{jk}$, $\epsilon_{jl}$, and $\epsilon_{kl}$ are below $\mathscr{C}$. Following to $n = 4$, two 3-body terms are above $\mathscr{C}$ ($\epsilon_{ijk}$ and $\epsilon_{ijl}$), so the 4-body term ($\epsilon_{ijkl}$) is connected, and therefore computed. Case 2 is an alternate example where one fewer of the 2-body terms is above $\mathscr{C}$, leading to only one computed 3-body term ($\epsilon_{ijk}$). The 4-body term in case 2 is also not computed, as it is only connected to the single 3-body term.

In the present work, we use a cutoff of $\mathscr{C} = 10^{-4.6}$ Ha (~25 μHa) for all calculations on PFAS. This value of $\mathscr{C}$ was made tighter than that used in Ref. 1 and 2 to capture contributions to the correlation from mid-range orbital interactions present in PFAS (in large part due to the many lone pairs).

## II. Total Number of *n*-Body Terms Computed

Utilizing the screening procedure detailed above with $\mathscr{C}=10^{-4.6}$ Ha, the total number of *n*-body terms computed for the reported BDE of each PFAS is shown in the table below. All listed values are for the equilibrium geometry, though the count of terms for the dissociated geometries are similar. For n=3 and 4, the ratio given is the number of terms computed versus the total number of terms, accompanied by the percentage of the total in parentheses. Note, we also performed a more rigorous exploration of the 3- and 4-body correlation of PFOA using a tighter screening value of $\mathscr{C}=10^{-6.0}$ Ha, producing the total of 416,857 4-body terms reported in the main text (218,670 for the equilibrium geometry and 198,187 for the dissociated geometry).

| PFAS | n=1 | n=2 | n=3 | n=4 |
|---|---|---|---|---|
| TFA | 21 | 210 | 1,222 / 1,330 (92%) | 1,906 / 5,985 (32%) |
| PFBA | 39 | 741 | 4,533 / 9,139 (50%) | 4,838 / 82,251 (6%) |
| PFOA | 75 | 2775 | 11,739 / 67,525 (17%) | 11,560 / 1,215,450 (1%) |

## III. Molecular Geometries

The equilibrium geometries for TFA, PFBA, and PFOA were obtained with optimization under the DF-MP2/cc-pVTZ level of theory. The rigid body scan of C–F changes only the coordinates of the bolded fluorine, where substituting one fluorine (marked bold) in the equilibrium geometries (1.3Å) with those listed in the accompanying tables forms each geometry studied in this work. All geometries are reported in Ångstrom.

Equilibrium TFA:

| | | | |
|---|---|---|---|
| C | 0.000000000000000 | 0.000000000000000 | 0.000000000000000 |
| F | 1.336794000000000 | 0.000000000000000 | 0.000000000000000 |
| C | -0.534720512610771 | 0.000000000000000 | 1.444607465513820 |
| O | -1.237839398622730 | -0.862893777617774 | 1.897868458658850 |
| F | -0.425397529055714 | -1.073476222919410 | -0.649990996544528 |
| **F** | **-0.419932971473614** | **1.089884253900700** | **-0.650251344485074** |
| O | -0.093892847399815 | 1.090615418331590 | 2.081639169894420 |
| H | -0.450368648651284 | 1.054253018038670 | 2.983751641014880 |

| C–F Bond Distance (Å) | TFA dissociated fluorine coordinates (all others remain the same as above) | | | |
|---|---|---|---|---|
| 0.9 | F | -0.294279214358123 | 0.763765419166046 | -0.455680948602066 |
| 1.0 | F | -0.325692653636996 | 0.845295127849710 | -0.504323547572818 |
| 1.1 | F | -0.357106092915868 | 0.926824836533375 | -0.552966146543570 |
| 1.2 | F | -0.388519532194741 | 1.008354545217030 | -0.601608745514322 |
| 1.3* | **F** | **-0.419932971473614** | **1.089884253900700** | **-0.650251344485074** |
| 1.4 | F | -0.451346410752487 | 1.171413962584360 | -0.698893943455826 |
| 1.5 | F | -0.482759850031359 | 1.252943671268030 | -0.747536542426578 |
| 1.6 | F | -0.514173289310232 | 1.334473379951690 | -0.796179141397330 |
| 1.7 | F | -0.545586728589105 | 1.416003088635360 | -0.844821740368082 |
| 1.8 | F | -0.577000167867978 | 1.497532797319020 | -0.893464339338834 |
| 1.9 | F | -0.608413607146850 | 1.579062506002680 | -0.942106938309586 |
| 2.0 | F | -0.639827046425723 | 1.660592214686350 | -0.990749537280338 |
| 2.1 | F | -0.671240485704596 | 1.742121923370010 | -1.039392136251090 |
| 2.2 | F | -0.702653924983469 | 1.823651632053680 | -1.088034735221840 |
| 2.3 | F | -0.734067364262342 | 1.905181340737340 | -1.136677334192590 |
| 2.4 | F | -0.765480803541214 | 1.986711049421010 | -1.185319933163340 |
| 2.5 | F | -0.796894242820087 | 2.068240758104670 | -1.233962532134090 |
| 2.6 | F | -0.828307682098960 | 2.149770466788340 | -1.282605131104850 |
| 2.7 | F | -0.859721121377833 | 2.231300175472000 | -1.331247730075600 |
| 2.8 | F | -0.891134560656705 | 2.312829884155660 | -1.379890329046350 |
| 2.9 | F | -0.922547999935578 | 2.394359592839330 | -1.428532928017100 |

| | |
|---|---|
| 3.0 | F -0.953961439214451 2.475889301522990 -1.477175526987850 |
| 3.5 | F -1.111028635608810 2.883537844941310 -1.720388521841610 |
| 4.0 | F -1.268095832003170 3.291186388359640 -1.963601516695370 |
| 4.5 | F -1.425163028397540 3.698834931777960 -2.206814511549130 |
| 5.0 | F -1.582230224791900 4.106483475196280 -2.450027506402890 |
| 5.5 | F -1.739297421186270 4.514132018614600 -2.693240501256650 |
| 6.0 | F -1.896364617580630 4.921780562032920 -2.936453496110410 |

Equilibrium PFBA:

| | | | |
|---|---|---|---|
| C | 0.00000000000000 | 0.00000000000000 | 0.00000000000000 |
| F | 1.33025600000000 | 0.00000000000000 | 0.00000000000000 |
| F | -0.43171203055332 | 0.00000000000000 | 1.25913461806890 |
| C | -0.53835381534556 | -1.26428503094711 | -0.71076087454708 |
| F | -1.87820916955892 | -1.13744718445738 | -0.81451595348117 |
| F | -0.43686185348877 | 1.10216733161831 | -0.59882143357157 |
| C | 0.03337770781569 | -1.52056744457512 | -2.12418750327200 |
| **F** | **1.31587501340936** | **-1.90383158331549** | **-2.01517808219031** |
| F | -0.26142066308452 | -2.32705730545313 | 0.05998493137409 |
| C | -0.75690405420368 | -2.64456218939313 | -2.82460560298819 |
| O | -1.68854556605018 | -2.14176794254888 | -3.64017670099600 |
| F | -0.02011362953580 | -0.37595132095380 | -2.83231321004973 |
| O | -0.53596965383349 | -3.80861506902844 | -2.61581280558891 |
| H | -2.16093777009582 | -2.90033284190621 | -4.02115424275392 |

| C–F Bond Distance (Å) | PFBA dissociated fluorine coordinates (all others remain the same as above) |
|---|---|
| 1.3* | **F 1.31587501340936 -1.90383158331549 -2.01517808219031** |
| 6.0 | F 5.80423168524636 -3.24514134411448 -1.63367773885928 |

Equilibrium PFOA:

| | | | |
|---|---|---|---|
| C | 0.00000000000000 | 0.00000000000000 | 0.00000000000000 |
| F | 1.33125900000000 | 0.00000000000000 | 0.00000000000000 |
| C | -0.53563518999579 | 0.00000000000000 | 1.45479514557863 |
| F | -0.29118914812952 | 1.20976612107189 | 1.98011542621091 |
| F | -0.43240672573550 | 1.09801594744037 | -0.61333433321910 |
| F | -0.43822513894639 | -1.06034682964760 | -0.66786539983419 |
| C | 0.11402708794949 | -1.08275782147589 | 2.35868159809783 |
| F | 1.33905328285720 | -0.65870599029981 | 2.71455629415129 |

| | | | |
|---|---|---|---|
| F | -1.86479830971494 | -0.20031832654331 | 1.39972473764182 |
| C | -0.71528595245900 | -1.37029984163301 | 3.64229697599784 |
| F | -1.17302225470322 | -0.20485140709508 | 4.12979171265133 |
| F | 0.23052049529984 | -2.22165737314657 | 1.65395405723667 |
| C | 0.11606746522609 | -2.08233154172213 | 4.74706505273274 |
| F | 0.89882608659971 | -1.17254518673249 | 5.35069223296564 |
| F | -1.75638637903898 | -2.15401390773321 | 3.31157344168609 |
| C | -0.77509057500038 | -2.76485201076944 | 5.82073147192268 |
| F | -1.24281260351991 | -3.92761822347503 | 5.32125312148408 |
| F | 0.88829545561955 | -3.01880384751716 | 4.16888119187459 |
| C | -0.02543688466741 | -3.08985456131413 | 7.13807300406596 |
| **F** | **0.14832798609383** | **-1.96113033999339** | **7.84349565954933** |
| F | -1.81486168972271 | -1.96495702971707 | 6.10862686840774 |
| C | -0.85982230603308 | -4.07192667624401 | 7.98543087763451 |
| O | -0.40744676069760 | -5.32310829999637 | 7.86374440187470 |
| F | 1.17996691556315 | -3.60849534084434 | 6.83509648271982 |
| O | -1.80059219085476 | -3.70708981526145 | 8.64096243859094 |
| H | -0.99519464607779 | -5.88233278931769 | 8.39822686573523 |

| C–F Bond Distance (Å) | PFOA dissociated fluorine coordinates (all others remain the same as above) | | | |
|---|---|---|---|---|
| 1.3* | **F** | **0.14832798609383** | **-1.96113033999339** | **7.84349565954933** |
| 6.0 | F | 0.75674658888855 | 1.99097350394257 | 10.31345558038200 |

## IV. References

[1] A. E. Rask and P. M. Zimmerman, Toward Full Configuration Interaction for Transition-Metal Complexes. *J. Phys. Chem. A* **125**, 1598-1609 (2021).
[2] A. E. Rask and P. M. Zimmerman, The Many-Body Electronic Interactions of Fe(II)-Porphyrin. *J. Chem. Phys.* **156**, 094110 (2022).
